# Supplementary material for: Farmer.Chat: Scaling AI-Powered Agricultural Services for Smallholder Farmers
Source: arXiv:2409.08916 source file (2024-10-08)
Supplement: Supplementary file 1 [file 8-appendix.tex]

\section{Appendix}

\section{Farmer.Chat Application Screenshot}

ADD telegram BOT images here and have few sentences.
